# Supplementary material for: Constraining the temperature-density relation of the intergalactic medium with the Lyman-$\alpha$ and $\beta$ forests
Source: arXiv:1510.08857 ancillary file (2015-11-07)
Supplement: Supplementary file 1 [file SupportingInformation.pdf]

**Table 1.** Quasars used for this analysis. Column 1 shows the quasar names and column 2 shows their emission redshifts. The note below the table provides the ESO Program IDs that contributed to the spectra.

| Quasars        | $z_{em}$ |
|----------------|----------|
| J110325–264515 | 2.145    |
| J012417–374423 | 2.2004   |
| J145102–232930 | 2.215    |
| J024008–230915 | 2.223    |
| J212329–005052 | 2.2623   |
| J000344–232355 | 2.28     |
| J045313–130555 | 2.30     |
| J112442–170517 | 2.40     |
| J222006–280323 | 2.406    |
| J011143–350300 | 2.41     |
| J033106–382404 | 2.423    |
| J120044–185944 | 2.448    |
| J234628+124858 | 2.515    |
| J015327–431137 | 2.74     |
| J235034–432559 | 2.885    |
| J040718–441013 | 3.00     |
| J094253–110426 | 3.054    |
| J042214–384452 | 3.11     |
| J103909–231326 | 3.13     |
| J114436+095904 | 3.15     |
| J212912–153841 | 3.268    |
| J233446–090812 | 3.3169   |
| J010604–254651 | 3.365    |
| J014214+002324 | 3.3714   |
| J115538+053050 | 3.4752   |
| J005758–264314 | 3.655    |
| J014049–083942 | 3.7129   |

ESO Program IDs: 60.A-9022, 60.A-9207, 60.O-9025, 65.O-0063, 65.O-0158, 65.O-0296, 65.O-0299, 65.O-0474, 65.P-0038, 65.P-0183, 66.A-0133, 66.A-0212, 66.A-0221, 66.A-0624, 67.A-0022, 67.A-0078, 67.A-0146, 67.A-0280, 67.B-0398, 68.A-0170, 68.A-0216, 68.A-0230, 68.A-0361, 68.A-0461, 68.A-0570, 68.A-0600, 68.B-0115, 69.A-0204, 69.B-0108, 70.A-0017, 70.B-0258, 71.A-0066, 71.A-0067, 71.B-0106, 71.B-0136, 072.A-0100, 072.A-0346, 072.A-0446, 072.A-0446, 072.B-0218, 073.B-0420, 073.B-0787, 075.A-0464, 075.B-0190, 076.A-0376, 076.A-0463, 076.A-0860, 077.A-0646, 078.A-0003, 079.A-0108, 079.A-0251, 079.A-0303, 079.A-0404, 079.B-0469, 080.A-0014, 080.A-0482, 080.A-0795, 081.A-0242, 081.B-0285, 166.A-0106, 267.A-5714, 273.A-5020.

## References

- Becker G. D., Bolton J. S., Haehnelt M. G., Sargent W. L. W., 2011, MNRAS, 410, 1096  
 Boera E., Murphy M. T., Becker G. D., Bolton J. S., 2014, MNRAS, 441, 1916  
 Haardt F., Madau P., 2001, in Clusters of Galaxies and the High Redshift Universe Observed in X-rays, Neumann D. M., Tran J. T. V., eds.

**Table 2.** Parameters corresponding to the different simulations used in this work. We adopted the same simulations originally made for the work of Becker et al. (2011) and extended towards lower redshift for the work of Boera et al. (2014). For each simulation we report the name of the model (column 1), the constants used to rescale the photo-heating rates for the different thermal histories (columns 2 & 3), the temperature of the gas at the mean density at  $z = 3$  (column 4) and the power-law index of the  $T$ - $\rho$  relation at  $z = 3$  (column 5). In particular, for the different species ( $i$ =[H I, He I, He II]) the photo-heating rates from Haardt & Madau (2001) ( $\epsilon_i^{HM01}$ ) have been modified following the prescription  $\epsilon_i = \zeta \Delta^\xi \epsilon_i^{HM01}$  where  $\epsilon_i$  are the adopted photo-heating rates and  $\zeta$  and  $\xi$  are constants that change depending on the thermal history assumed.

| Model | $\zeta$ | $\xi$ | $T_0^{z=3}$ [K] | $\gamma^{z=3}$ |
|-------|---------|-------|-----------------|----------------|
| A15   | 0.30    | 0.00  | 5100            | 1.52           |
| C15   | 1.45    | 0.00  | 14000           | 1.54           |
| D15   | 2.20    | 0.00  | 18200           | 1.55           |
| E15   | 3.10    | 0.00  | 22500           | 1.55           |
| F15   | 4.20    | 0.00  | 27000           | 1.55           |
| G15   | 5.30    | 0.00  | 31000           | 1.55           |
| D13   | 2.20    | -0.45 | 18100           | 1.32           |
| C10   | 1.45    | -1.00 | 13700           | 1.02           |
| D10   | 2.20    | -1.00 | 18000           | 1.03           |
| E10   | 3.10    | -1.00 | 22200           | 1.04           |
| D07   | 2.20    | -1.60 | 17900           | 0.71           |

**Table 3.** Parameters corresponding to the different simulations used in the curvature ratio convergence tests in Figure 1 of the SI. For each simulation we report the name of the model (column 1), the box size (column 2), the total number of particles and their mass (column 3 & 4). All the simulations were run with the same thermal history assumption as in model C15.

| Model | $L[h^{-1}\text{Mpc}]$ | Particles        | $M_{\text{gas}}[h^{-1}M_\odot]$ |
|-------|-----------------------|------------------|---------------------------------|
| C15   | 10                    | $2 \times 512^3$ | $9.2 \times 10^4$               |
| R1    | 10                    | $2 \times 256^3$ | $7.4 \times 10^5$               |
| R2    | 10                    | $2 \times 128^3$ | $5.9 \times 10^6$               |
| R3    | 20                    | $2 \times 256^3$ | $5.9 \times 10^6$               |
| R4    | 40                    | $2 \times 512^3$ | $5.9 \times 10^6$               |

**Table 4.** Parameters corresponding to the different fits of the  $\gamma$ - $\log(R_k)$  relationship at different redshifts. The general fitting function is a simple power-law:  $\log(R_k) = a\gamma^b + c$ . For each redshift (column 1) we report the parameter  $a$  (column 2),  $b$  (column 3) and  $c$  (column 4). The corresponding fits are shown in Figure 2 of the SI. Note these parameters apply only to the simulations used in this work.

| $z$   | $a$    | $b$   | $c$   |
|-------|--------|-------|-------|
| 2.173 | -0.248 | 1.265 | 0.296 |
| 2.355 | -0.186 | 1.393 | 0.250 |
| 2.553 | -0.111 | 1.786 | 0.186 |
| 2.760 | -0.083 | 2.033 | 0.172 |
| 3.211 | -0.034 | 3.038 | 0.135 |
| 3.457 | -0.029 | 3.187 | 0.141 |

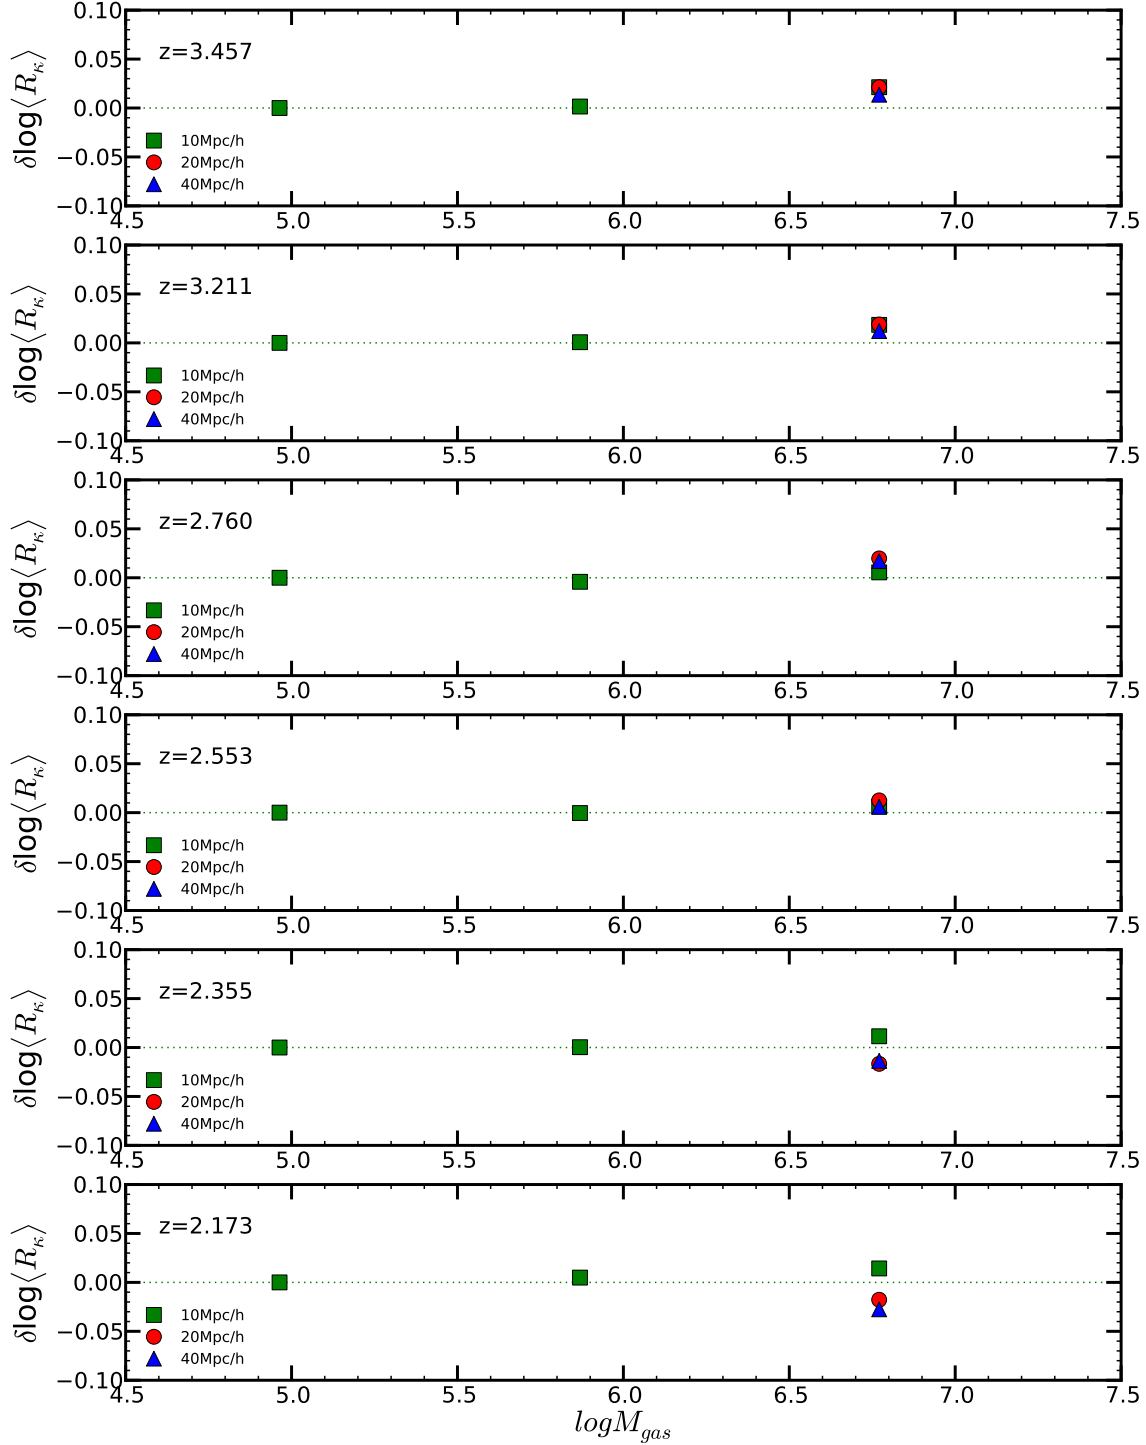

**Figure 1.** Convergence of the mean curvature ratio with box size and mass resolution. Curvature ratio values were computed from noise-free spectra, using the same procedure described in Section 4.1. The change in  $\log\langle R_k \rangle$  is plotted with respect to the model with the best mass resolution (model C15 from the nominal suite of simulations of Table 2). The results show that this statistic is well converged with mass resolution at all redshifts: for a fixed  $10h^{-1}\text{Mpc}$  box size (green squares) there are not significant differences in terms of mass resolution, with variations  $\delta\log\langle R_k \rangle \lesssim 0.02$  for all the models presented. In the lowest resolution case, the vertical separation between the data points allows us to judge the box size convergence and shows good convergence for  $z \gtrsim 2.3$ . The largest variation is at  $z = 2.173$ , where the decrease in  $\log\langle R_k \rangle$  when increasing the box size from  $10h^{-1}\text{Mpc}$  to  $40h^{-1}\text{Mpc}$  would correspond to a small change ( $\lesssim 5$  per cent) in the final  $\gamma$  measurements.

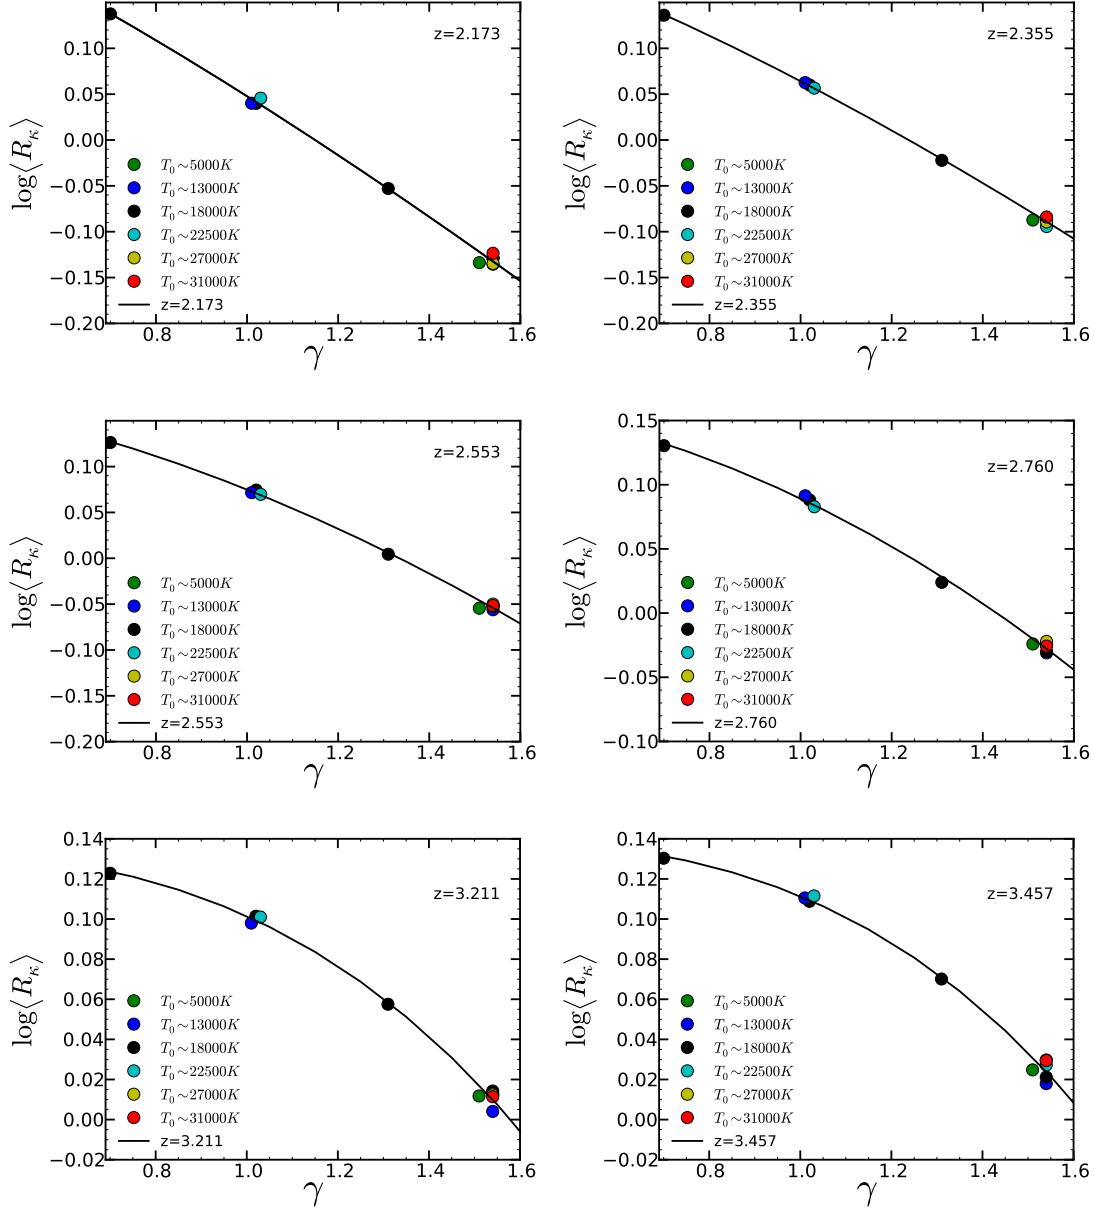

**Figure 2.** Relationship between the slope parameter of the temperature–density relation,  $\gamma$ , and the curvature ratio,  $R_k$ , from our nominal simulations. Each panel shows the relationship at a particular redshift, obtained from synthetic spectra with different thermal histories. At each redshift, the values of  $\log\langle R_k \rangle$  for the different models presented in Table 2 (coloured points) lie on the same curve, with little sensitivity to differences in  $T_0$ . Each solid line represents the least square fit of the  $\log\langle R_k \rangle$  values. The fit parameters for each redshift are given in Table 4.

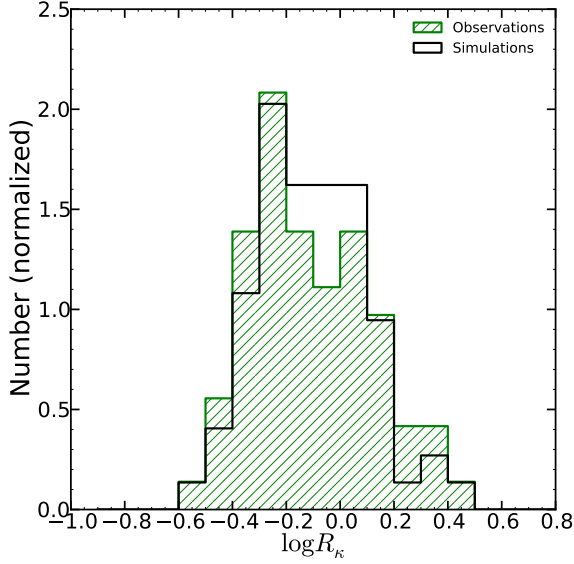

**Figure 3.** Comparison between the shape of the  $\log R_k$  distribution observed in the lowest redshift bin (green histogram) and the distribution obtained from the simulation model F15 at  $z = 2.355$  (black histogram). Both the distributions have been normalized (i.e. the integral of each histogram is equal to 1) for the comparison and show similar Gaussian shapes and widths. This agreement provides some confidence that the dispersion in our measurements of  $\log R_k$  is well reproduced by the simulations used in this work.

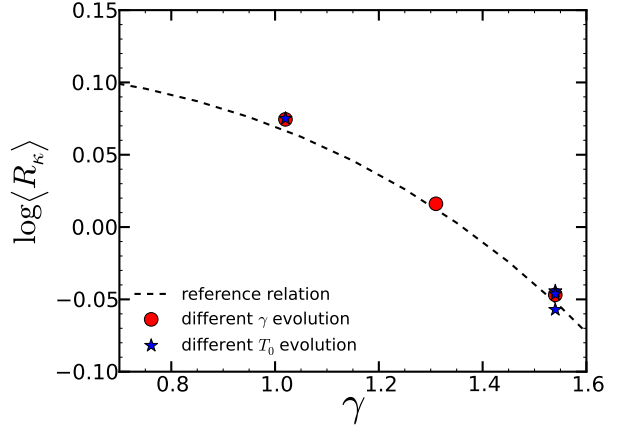

**Figure 4.** Sensitivity of the  $\gamma$ – $\log\langle R_k \rangle$  relation to the Jeans smoothing effect. To test the sensitivity of the  $\gamma$ – $\log\langle R_k \rangle$  relation to variations in the integrated thermal history we can apply modifications to the density distribution of the absorbers (i.e. overdensity distribution) in the simulations using a post-processing approach similar to that in Section 4.3. Firstly, for each simulation model of Table 2 we impose a one-to-one power-law  $T$ – $\rho$  relationship in which we maintain the original density fields of the nominal simulations. From the  $\log\langle R_k \rangle$  values computed from these models we then obtain a “reference”  $\gamma$ – $\log\langle R_k \rangle$  relation (black dashed line). Secondly, for few cases, holding fixed the “instantaneous” values of  $T_0$  and  $\gamma$  at each redshift, we substitute the density fields of one nominal simulation for the density fields of another, evolved with a different thermal history, i.e. with different  $T_0$  (blue stars) or  $\gamma$  (red dots). In particular, in the case of different  $T_0$  values we substitute the density fields of the model D15 for the ones of the model C15 and for the ones of the model G15 and we substitute the density fields of the model D10 for the ones of the model C10. In the case of different  $\gamma$  values we substitute the density fields of the model D15 for the ones of the model D13, the density fields of D13 for the ones of D10 and finally the density fields of the model D10 for the ones of the model D07. Any difference between the  $\log\langle R_k \rangle$  computed from the new extracted spectra and those from the reference ones will then only be due to differences in the overdensity distribution and, consequently, to the Jeans smoothing effect. In all cases, the values of  $\log\langle R_k \rangle$  do not seem to depart significantly from the reference relation.
